# Supplementary material for: Combinatorial Parameterized Algorithms for Chemical Descriptors based on Molecular Graph Sparsity
Source: arXiv:2303.13279 source file (2025-08-11)
Supplement: Supplementary file 1 [file old-appendix.tex]

% !TEX root = ../main.tex

\section{Appendix}
\subsection{Fast counting perfect matching in chain graphs}
Now we consider class of graphs obtained by chain repetition of one small graph. We are calling such graph as a chain, and small graph as a chain element. For examples see fig. ??. 

\begin{definition}
	\textit{Chain element} is a fixed graph $G$ with two selected vertices subsets $L(G), R(G) \subset V(G)$ and bijection between them $f: L(G) \rightarrow R(G)$ such that graph induced from $G$ to $L(G)$ is isomorphic to graph induced from $G$ to $R(G)$ via isomorphism $f$. 
	
	It will be convinient to denote $k = \lvert{V(G)}\rvert$ and set $V(G) = \{v_1, \dots, v_k\}$.
\end{definition}

Using this properties it is easy to chain them sequentially.  

\begin{definition}
	Chain graph of length $n$ obtained from chain element $G$ denoted as $\textup{chain}(G, n)$ is a graph obtained from $n$ disjunctive copies of $G$: $\{G^1, G^2, \dots, G^n\}$ by identifying $R(G^i)$ with $L(G^{i + 1})$ via isomorphism $f$ for each $i\in [1, n - 1]$.
	
	Vertex set in each graph $G^i$ we are denoting as $\{v_1^i, \dots, v_k^i\}$.  
\end{definition}

Now to count perfect matchings in chain graph, we will use dynamic programming. This dynamic programming parameterized by two parameters:
\begin{enumerate}
	\item Length of chain $n \in \mathbf{N}$,
	\item Vertex subsets of $G \setminus L(G)$ : 
	$$I = \{S: S \subset G\setminus L(G)\}.$$
	For example in fig ?? we have 
	$$I = \{S: S \subset\{v_1, v_2, v_3, v_4\}\setminus \{v_1, v_2\}\} = \{\varnothing, \{v_3\}, \{v_4\}, \{v_3, v_4\}\}.$$
\end{enumerate}

Second dynamic programming parameter playing role of vertices, that not matched on step $i$, but will be matched on a step $i + 1$.

Formally let us fix natural number $n \in \mathbf{N}$ and second index $\alpha \in I$. Then:
$$
	b_{n, \alpha} = \textup{\#PM}(\textup{chain}(G, n) \setminus \alpha^n),
$$
where $\alpha^n$ is upper-indexing of verticies from $\alpha$ with index $n$.

Now we need to establish recurrence relations which relate $b_{n, *}$ to $b_{n - 1, *}$.

Consider any vertex from $v \in G^n \setminus(L(G^n)\cup \alpha^n)$. It should be covered by some edge $e$. Because set $L(G^n)$ separates graphs $G^n$ and $\textup{chain}(G, n - 1)$, second end of edge $e$ must end also in $G^n$. So to compute $b_{n, \alpha}$, we need consider all partial matchings such that each edge from matching has endpoint in $G^n \setminus(L(G^n)\cup \alpha^n)$ and all vertices $G^n \setminus(L(G^n)\cup \alpha^n)$ are covered and each edge from matching does not have endpoint in $\alpha^n$. Lets call set of such partial matchings $\mathcal{M}_{n, \alpha}$. Because of $L(G)$ separation property we mentioned before, each matching contains in $G^n$: $\forall M \in \mathcal{M}_{n, \alpha}: M \subset G^n$, so it is easy to enumerate them in $\textup{poly}(\lvert V(G)\rvert)$ time. And our recurrence relation is:
$$
b_{n, \alpha} = \sum\limits_{M \in \mathcal{M}_{n, \alpha}} b_{n - 1, \textup{EraseUpperIndices}(f^{-1}(G^{n - 1} \cap M))}.
$$ 

Notice that all sets $\mathcal{M}_{n, \alpha}$ do not depend on $n$ (up to erasure of upper indices). So our relations also are same and could be expressed in matrix form:
$$
(b_{n, \varnothing}, \dots, b_{n, G\setminus L(G)})^{\top} = A\cdot(b_{n - 1, \varnothing}, \dots, b_{n - 1, G\setminus L(G)})^{\top},
$$ 
where $A$ is $2^{G\setminus L(G)}\times 2^{G\setminus L(G)}$ matrix with 

\begin{align*}
	a_{\alpha, \alpha^\prime} = \#\{M \in \mathcal{M}_{\alpha}: 
	&(\forall e \in M. e \cap G \setminus(\alpha \cup \alpha^\prime) \neq \varnothing)\\
	& \wedge (\forall v \in G \setminus (\alpha \cup \alpha^\prime).v\in V(M)) \\ 
	& \wedge M \cap \alpha^\prime = \varnothing \}.
\end{align*}

Now to compute $b_{n, *}$ we only need to multiply $b_{1, *}$ by matrix $A$ $(n - 1)$ times: 
$$
(b_{n, \varnothing}, \dots, b_{n, G\setminus L(G)})^{\top} = A^{n - 1}\cdot(b_{1, \varnothing}, \dots, b_{1, G\setminus L(G)})^{\top}.
$$ 

Now we came to main observation. We can find $A^{n - 1}$ using only $\log_2(n - 1)$ matrix multiplication!

So overall complexity is complexity for building matrix $A$ which is negligible plus $(2^{G \setminus L(G)})^\omega \times \log_2(n)$, where $\omega$ is optimal matrix multiplication constant. 

\subsection{Example}

In this section we show how to compute number of perfect matchings in a chain graph, with chain element is cycle of length $6$ 

\begin{align*}
C_6 = \{
&V = \{v_1, v_2, v_3, v_4, v_5, v_6\},\\
& E = \{\{v_1, v_2\}, \{v_2, v_3\}, \{v_3, v_4\}, \{v_4, v_5\}, \{v_5, v_6\}, \{v_6, v_1\}\}\},
\end{align*}
with 
\begin{align*}
&L(C_6) = \{v_1, v_2\},\\
&R(C_6) = \{v_4, v_5\},
\end{align*}

isomorphism map is $f(v_1) = v_5, f(v_2) = v_6$,
see ?? for illustration. 

Then in previous chapter definition:


\begin{align*}
I = \{
 &\varnothing, \{v_3\}, \{v_4\}, \{v_5\}, \{v_6\},\\
 &\{v_3, v_4\}, \{v_3, v_5\}, \{v_3, v_6\}, \{v_4, v_5\}, \{v_4, v_6\}, \{v_5, v_6\}, \\
 &\{v_3, v_4, v_5, v_6\}, \{v_3, v_4, v_5, v_6\}, \{v_3, v_4, v_5, v_6\}, \{v_3, v_4, v_5, v_6\}\}.
\end{align*}

Instead of writing $b_{n, \{v_2, v_4\}}$ we will omit $v$ and write $b_{n, 24}$ instead. Now we need to write relations. For $\alpha = \varnothing$ we have two way of matching vertices $\{v_3, v_4, v_5, v_6\}$: $\{\{v_3, v_4\}, \{v_5, v_6\}\}$ and $\{\{v_1, v_2\}, \{v_3, v_4\}, \{v_5, v_6\}\}$. In first case vertices $\{v_1, v_2\}$ remains uncovered, so we need to take $f^{-1}$ of them to get $\{v_4, v_5\}$. In second case all vertices are covered, so $f^{-1}(\varnothing) = \varnothing$, finally relation is:
$$
v_{n, \varnothing} = v_{n - 1, \varnothing} + v_{n - 1, 45}. 
$$ 

Other relations omitting symmetries:

\begin{align*}
&b_{n, 3} = b_{n - 1, 4},\\
&b_{n, 4} = b_{n - 1, 5},\\
&b_{n, 34} = b_{n - 1, \varnothing}, \\
&b_{n, 35} = 0,\\
&b_{n, 36} = b_{n - 1, \varnothing}, \\
&b_{n, 45} = b_{n - 1, 45}, \\
&b_{n, 345} = b_{n - 1, 4}, \\
&b_{n, 346} = 0, \\
&b_{n, 3456} = b_{n - 1, \varnothing}.
\end{align*}
	
Then transition matrix is:
\setcounter{MaxMatrixCols}{20}
$$
\begin{pmatrix}
b_{n, \varnothing} \\
b_{n, 3} \\
b_{n, 4} \\
b_{n, 5} \\
b_{n, 6} \\
b_{n, 34} \\
b_{n, 35} \\
b_{n, 36} \\
b_{n, 45} \\
b_{n, 46} \\
b_{n, 56} \\
b_{n, 345} \\
b_{n, 346} \\
b_{n, 356} \\
b_{n, 456} \\
b_{n, 3456} \\
\end{pmatrix}
=
\begin{pmatrix}
b_{n - 1, \varnothing} \\
b_{n - 1, 3} \\
b_{n - 1, 4} \\
b_{n - 1, 5} \\
b_{n - 1, 6} \\
b_{n - 1, 34} \\
b_{n - 1, 35} \\
b_{n - 1, 36} \\
b_{n - 1, 45} \\
b_{n - 1, 46} \\
b_{n - 1, 56} \\
b_{n - 1, 345} \\
b_{n - 1, 346} \\
b_{n - 1, 356} \\
b_{n - 1, 456} \\
b_{n - 1, 3456} \\
\end{pmatrix}
\begin{pmatrix}
1 & 0 & 0 & 0 & 0 & 0 & 0 & 0 & 1 & 0 & 0 & 0 & 0 & 0 & 0 & 0\\
0 & 0 & 0 & 1 & 0 & 0 & 0 & 0 & 0 & 0 & 0 & 0 & 0 & 0 & 0 & 0\\
0 & 0 & 1 & 0 & 0 & 0 & 0 & 0 & 0 & 0 & 0 & 0 & 0 & 0 & 0 & 0\\
0 & 0 & 0 & 1 & 0 & 0 & 0 & 0 & 0 & 0 & 0 & 0 & 0 & 0 & 0 & 0\\
0 & 0 & 1 & 0 & 0 & 0 & 0 & 0 & 0 & 0 & 0 & 0 & 0 & 0 & 0 & 0\\
1 & 0 & 0 & 0 & 0 & 0 & 0 & 0 & 0 & 0 & 0 & 0 & 0 & 0 & 0 & 0\\
0 & 0 & 0 & 0 & 0 & 0 & 0 & 0 & 0 & 0 & 0 & 0 & 0 & 0 & 0 & 0\\
1 & 0 & 0 & 0 & 0 & 0 & 0 & 0 & 0 & 0 & 0 & 0 & 0 & 0 & 0 & 0\\
0 & 0 & 0 & 0 & 0 & 0 & 0 & 0 & 1 & 0 & 0 & 0 & 0 & 0 & 0 & 0\\
0 & 0 & 0 & 0 & 0 & 0 & 0 & 0 & 0 & 0 & 0 & 0 & 0 & 0 & 0 & 0\\
1 & 0 & 0 & 0 & 0 & 0 & 0 & 0 & 0 & 0 & 0 & 0 & 0 & 0 & 0 & 0\\
0 & 0 & 0 & 1 & 0 & 0 & 0 & 0 & 0 & 0 & 0 & 0 & 0 & 0 & 0 & 0\\
0 & 0 & 0 & 0 & 0 & 0 & 0 & 0 & 0 & 0 & 0 & 0 & 0 & 0 & 0 & 0\\
0 & 0 & 0 & 0 & 0 & 0 & 0 & 0 & 0 & 0 & 0 & 0 & 0 & 0 & 0 & 0\\
0 & 0 & 1 & 0 & 0 & 0 & 0 & 0 & 0 & 0 & 0 & 0 & 0 & 0 & 0 & 0\\
1 & 0 & 0 & 0 & 0 & 0 & 0 & 0 & 0 & 0 & 0 & 0 & 0 & 0 & 0 & 0\\
\end{pmatrix},
$$
and initial assignment is
$$
\begin{pmatrix}
b_{1, \varnothing} \\
b_{1, 3} \\
b_{1, 4} \\
b_{1, 5} \\
b_{1, 6} \\
b_{1, 34} \\
b_{1, 35} \\
b_{1, 36} \\
b_{1, 45} \\
b_{1, 46} \\
b_{1, 56} \\
b_{1, 345} \\
b_{1, 346} \\
b_{1, 356} \\
b_{1, 456} \\
b_{1, 3456} \\
\end{pmatrix}
=
\begin{pmatrix}
2\\
0\\
0\\
0\\
0\\
1\\
0\\
1\\
1\\
0\\
1\\
0\\
0\\
0\\
0\\
1\\
\end{pmatrix},
$$


\begin{figure*}[h]
	\centering
	\includegraphics{./chapters/images/hexagons.pdf}
\end{figure*}

\section{Counting Independent Sets}

Will use a dynamic programming over the nice tree decomposition in a bottom-up manner. Let us fix a nice tree decomposition $\mathcal{T} = \{T, \{X_t\}_{t \in V(T)}\}$. For each node $b$ and each subset of a bag $M \subset X_b$ we define $\dpt[b, M]$ as a number of independent sets in a $G_b^\downarrow$ such that each independent set $I \subseteq V(G_b^\downarrow) \setminus X_b$ and $N_{G_b^\downarrow}(I) \cap X_b = X_b \setminus M$. We call such independent set \textit{respectful} to the $(X_b, M)$.


If $X_l = \varnothing$ is a leaf bag, we have only empty $(X_l, \varnothing)$-respectful independent set, which means 
\[
\dpt[X_l, \varnothing] = 1.
\]

Also for the root bag $X_r$, $\dpt[X_r, \varnothing]$ contains number of independent sets in a whole graph $G$.

Now we need to consider three cases of tree decomposition nodes: introduce node, forget node and merge node. 

\textbf{Introduce case.} Let $X_b$ is an introduce bag which introduces vertex $v$, let its child is a bag $X_c$, $X_b = X_c \cup \{v\}$. Then

\[
\dpt[b,M]=
\begin{cases}
dp[c,M \setminus v], & v \in M\\
0,                   & v\notin M.
\end{cases}
\]

Indeed, if $v \notin M$, each $(X_b, M)$-respectful independent set $I$ is $I \subset G_b^\downarrow \setminus X_b \subseteq G_c^\downarrow \setminus X_c$, therefore by lemma \ref{intseplemma} $N_{G_b^\downarrow}(v) \subseteq X_c$ and $N_{G_b^\downarrow}(v) \cap I = \varnothing$, which contradicts with the definition of $(X_b, M)$-respectfulness. 

If $v \in M$ then clearly each $(X_b, M)$-respectful independent set $I$ is an $(X_c, M \setminus v)$-respectful and vise versa. 


\textbf{Forget case.} Consider now a node $X_b$. Let $v$ be the vertex erased in $X_b$ and $X_c$ is a child of the $X_b$. Then


\[
\dpt[b, M] =
	\begin{cases}
	\begin{aligned}
		\dpt[c, M \cup v] &+ dp[c,M]\\
		&+ \sum_{H \subseteq X_c \cap N_{G_c^\downarrow}(v)} \dpt[c, M \cup H \cup v],
	\end{aligned} & N_{G_b^\downarrow}(v)\subseteq X_b\setminus M\\
\dpt[c, M \cup v] + dp[c,M], & 
N_{G_b^\downarrow}(v) \cap M \neq \varnothing.
	\end{cases}
\]

To prove this we need consider two cases: whether $N_{G_b^\downarrow}(v) \cap M = \varnothing$ or not. 

Consider the case when $N_{G_b^\downarrow}(v) \cap M = \varnothing$. Then each $(X_b, M)$-respectful set $I$ can either contain $v$ or not. If $v \notin I$ then two possible cases: either $v \in N_{c} ^\downarrow(I)$ or $v \notin N_{c} ^\downarrow(I)$. Depending the last conditions $I$ is an $(X_c, M \cup v)$ or $(X_c, M)$-respectful, which corresponds to the $\dpt[c, M \cup v]$ and $\dpt[c, M]$ terms. If $v \in I$ then $N_{G_c^\downarrow}(I \setminus v)$ must contain all non-neighbours of $v$ in $X_c \setminus M$ and maybe some neighbours $X_c \cap N_{G_c^\downarrow}(v)$. Brute such subsets we are getting our sum. 

In case $N_{G_b^\downarrow \neq \varnothing}$, each $(X_b, M)$-respectful independent set $I$ do not contain $v$, and we are having only first two terms similar to the first case. 


\textbf{Merge case}. Let $X_b$ is an merge bag and it has two children $X_{c_1}, X_{c_2}$, $X_b = X_{c_1} = X_{c_2}$. Then 
\[
\begin{aligned}
\dpt[b, M] 
&= \sum_{H_1 \sqcup H_2 \subseteq X_b \setminus M} \dpt[c_1, M\cup H_2] \cdot \dpt[c_, M \cup H_1]\\
&= \sum_{M_1 \subseteq X_b \setminus M}\sum_{M_2 \subseteq X_{b} \setminus(M \cup M_1)}\dpt[c_1,M\cup M_1]\cdot \dpt[c_2, M \cup M_2].
\end{aligned}
\]

This two sums are equivalent but first is easy to analyze and second is easy to implement. 

Consider $(X_b, M)$-respectful independent set $I$. Consider sets $I_1 := I \cap V(G_{c_1}^\downarrow)$ and $I_2 := I \cap V(G_{c_1}^\downarrow)$. It is evident that $I_1, I_2$ are independent sets in $G_{c_1}, G_{c_2}$ and they are $(X_{c_1}, M_1)$ and $(X_{c_2}, M_2)$-respectful for some $X_c \supseteq M_1, M_2 \supseteq M$. Now lemma \ref{joinseplemma} allow us to reverse this process: for each $X_c \supseteq M_1, M_2 \supseteq M$, each $(X_{c_1}, M_1)$-respectful set $I_1$ and $(X_{c_2}, M_2)$-respectful set $I_2$, they are disjoint $I_1 \cap I_2 = \varnothing$ (by the definition of respectfulness) and $I_1 \cup I_2$ are independent by lemma \ref{joinseplemma}.

\begin{proposition}
The overall complexity of filling $\dpt[b, \star]$ is $\bigO(4^\textup{tw})$ (because we need to split $X_b$ into four sets: $M$, $I_1$, $I_2$ and their complement $X_v \setminus \{M \cup M_1 \cup M_2\}$), and complexity of the whole algorithm is $\bigO(n \cdot 4^{\textup{tw}})$.
\end{proposition}


%\subsection{Counting Maximal Independent Sets}
%
%\subsubsection{Bounded Pathwidth}
%
%We will use a dynamic programming on the nice path decompositions.
%
%We will define the dynamic program as follows:
%\[\forall b \in B \text{ and } \forall M \subseteq v_b\]
%\[dp[b,M]:=\text{the number of maximal indepent sets $\textup{I}$ in $G_b^\downarrow-b$ s.t. $b \cap N(\textup{I})=(b-M)$}\]
%
%Where $G_b^\downarrow$ is the graph induced by the subtree of $b$. $M$ represents the vertices that can be added to the inpedendent set (vertices that are not in the independ set and are not neighbors of any vertex in the independent set).
%
%Let us consider how to recursively calculate the value of such dynamic program for each type of node in the tree decomposition. 
%
%Firstly an introduce node. Let $v$ be the vertex introduced in $b$ and $c$ be the child of $b$.
%\[dp[b,M]=
%\begin{cases}
%	dp[c,M-v], &v\in M\\
%	0,&v\not\in M
%\end{cases}\]
%
%This can be calculated in $O(1)$ time.
%
%Consider now an erase node. Let $v$ be the vertex erased in $b$ and $c$ be the child of $b$.
%
%\[dp[b,M]=
%	\begin{cases}
%		%nenhum vertice vizinho ta em mim -> eu posso estar no IS
%		dp[c,M] + \sum_{M'\subseteq N(v)} dp[c,M+M'+v], &N(v)\subseteq (b-M)\\
%		dp[c,M], &N(v)\not \subseteq (b-M)
%	\end{cases}
%\]
%
%This can be calculated in $O(k)$ time. Leaf nodes will always have value $1$, as there are not vertices to be matched.
%
%The final complexity is $\mathbf{O}(nk3^k)$
%
%\subsubsection{Bounded Treewidth}
%
%For bounded treewidth, we need to add the merge nodes. For them, we need to consider which child matched each \emph{matched} vertex. Let $c_1$ and $c_2$ be the children of bag $b$.
%
%
%\[dp[b,M]=\sum_{M_L \subseteq \overline{M}}\sum_{M_R \subseteq \overline{M \cup M_L}}dp[c_1,M+M_L]\cdot dp[c_2,M+M_R]\]
%
%With this, the final complexity of the algorithm increases to $O(nk4^k )$.
